# Supplementary material for: Opponent-aware Role-based Learning in Team Competitive Markov Games
Source: arXiv:2301.05873 source file (2023-01-14)
Supplement: Supplementary file 1 [file 400Appendix.tex]

\clearpage
\appendix
%{\huge Supplementary material}

%\vspace{-6mm}
\section{Pseudo Code of our algorithm}
\begin{algorithm}
	\caption{ \our\ }
	\label{modifiedAlgo}
	%	\KwData{$M$: \#episodes, $T$: max episode length, $N$: \#agents, $\tau$: classfier update interval, $C$ : Constant}
	Initialize $E$ parallel environments with $N$ agents\\
	Initialize replay buffer, $D$\\
	$T_{update} \leftarrow 0$\\
	\For{$i_{ep} = 1 \cdots $ max episodes}{
		$\tau_i^{0,e} \gets 0$\\
		$H_i^{0,e} \gets \emptyset, \forall i	$\\
		Reset all environments, and get initial $o_i^{1,e}$ for each agent $i$\\
		\For{$t=1 \cdots $ episode length }{
			In each environment $e$, sample roles for each agent $\rho_i^{t,e}, [\hat{\rho}^{t,e}_j]$ using eq.~(\ref{eq:roles})\\
			In each environment $e$, sample action from respective policies $a_i^{t,e} \sim \pi_i(o_i^{t,e},\rho_i^{t,e},[\hat{\rho}^{t,e}_j])$ \\
			Each agent receives $o_i^{t+1,e}, r_i^{t,e}$ from respective environments\\
			$\tau_i^{t,e} \gets \tau_i^{t-1,e} + (o_i^{t,e},a_i^{t,e})$\\
			$H_i^{e} \gets H_i^{e} + (o_i^{t,e},\tau_i^{t-1,e},a_i^{t,e},r_i^{t,e},o_i^{t+1,e})$\\
		}
		%		$H^e$ for all episodes, are stored in $D$\\
		$T_{update}=T_{update}+E$\\
		\If{$T_{update} \geq $ min steps per update}{
			\For{$j=1 \cdots $number of updates}{
				$H_B \gets B$ episodes sampled from $D$\\
				Update($H_B$,$\text{window length}$)\\
			}
			
			%	 		$\bar{\phi}=\tau \bar{\phi} + (1-\tau) \phi $ \tcc{Update critic parameters}
			%	 		$\bar{\theta}=\tau \bar{\theta} + (1-\tau) \theta $ \tcc{Update actor parameters}
			%	 		$\bar{\psi}= \psi $ \tcc{Update role parameters}
			$T_{update} \leftarrow 0$\\
		} 		 
	}
\end{algorithm}

\begin{algorithm}
	\caption{Update($H_B,\text{window length}$)}
	\label{update}
	Randomly select $t_1,\cdots, t_B$, the starting time-step for each of the $B$ episodes\\
	\For{$j = 1 \cdots \text{window length}$ }{
		$S \gets \emptyset$ \\
		\For{$k=1 \cdots B $}{
			$S \gets S  + (o_{1 \cdots N}^{t_k+j,k}, \tau_{1 \cdots N}^{t_k-1+j,k}, a_{1 \cdots N}^{t_k+j,k}, r_{1 \cdots N}^{t_k+j,k}, o_{1 \cdots N}^{t_k+1+j,k})$
		}
		$\rho^j,\hat{\rho}^j,\Lcal_{MI}^j,\Lcal_{D}^j, \Lcal_{Opp}^j \gets Role(S)$\\
		$\Lcal_{MI} \gets \Lcal_{MI} + \Lcal_{MI}^j,\Lcal_{D} \gets \Lcal_{D} + \Lcal_{D}^j, \Lcal_{Opp} \gets \Lcal_{Opp} + \Lcal_{Opp}^j$\\
		Update critics, policies and targets using $S, \rho^j, \hat{\rho}^j$\\
	}
	$\psi_{Role} \gets \argmin_{\psi}(\Lcal_{MI}+\Lcal_{D}+\Lcal_{Opp})$
\end{algorithm}
\begin{algorithm}
	\caption{Role($S$)}
	\label{role}
	Obtain roles $\rho_i^{t,e}, [\hat{\rho}_j^{t,e}]$ from eq. \ref{eq:roles} using for each agent $i$, environment $e$ from $S$\\
	$\rho^t \gets \rho_1^{t,\cdot} \cdots \rho_N^{t,\cdot},\hat{\rho}^{t} \gets \hat{\rho}_1^{t,\cdot} \cdots \hat{\rho}_N^{t,\cdot}$\\
	\For{$team = 1 \cdots \text{number of teams}$ }{
		\For{$agent=1 \cdots \text{number of agents in a team} $}{
			Calculate $\Lcal_{MI}$, $\Lcal_{D}$ and $\Lcal_{Opp}$ using eq. ~\ref{eq:miloss}, eq.~\ref{eq:dloss}, and eq.~\ref{eq:opp_loss}
		}
	}
	return $\rho^t,\hat{\rho}^t,\Lcal_{MI},\Lcal_{D},\Lcal_{Opp}$
\end{algorithm}
